# Supplementary material for: Decoupling of static and dynamic criticality in a driven Mott insulator
Source: arXiv:2112.08397 source file (2021-12-15)
Supplement: Supplementary file 1 [file SM_arxiv.pdf]

# Supplementary Information

# Decoupling of static and dynamic criticality in a driven Mott insulator

A. de la Torre[1,2], K. L. Seyler[1,2], M. Buchhold[1,2], Y. Baum[1,2], G. Zhang[3], N. J. Laurita[1,2], J. W. Harter[1,2], L. Zhao[1,2], I. Phinney[1,2], X. Chen[4,5], S. D. Wilson[5], G. Cao[6], R. D. Averitt[3], G. Refael[1,2] & D. Hsieh[1,2]

[1]*Department of Physics, California Institute of Technology, Pasadena, CA 91125, USA.*
[2]*Institute for Quantum Information and Matter, California Institute of Technology, Pasadena, CA 91125, USA.*
[3]*Department of Physics, University of California, San Diego, La Jolla, California 92093, USA*
[4]*Department of Physics, Boston College, Chestnut Hill, MA, 02467, USA*
[5]*Materials Department, University of California, Santa Barbara, CA, 93106, USA*
[6]*Center for Advanced Materials, Department of Physics and Astronomy, University of Kentucky, Lexington, Kentucky 40506, USA.*

Contents:

**S1.** **Effect of multiple layers on the measured magnetization dynamics**
**S2.** **Time-resolved SHG transients in the presence of a magnetic field**
**S3.** **Two- and three-temperature model results**
**S4.** **Coherent in-plane magnon in the $F > F_c$ regime**
**S5.** **Time-resolved SHG transients for $F > F^*$**
**S6.** **Ruling out alternative explanations for slow dynamics**
**S7.** **Details of the Langevin theory**
**S8.** **Restoration of the initial SHG-RA pattern after relaxation**
**S9.** **Time-resolved SHG transients for different polarization channels**

## S1. Effect of multiple layers on the measured magnetization dynamics

In this section we simulate how time-resolved transients differ depending on whether the probe is sensitive exclusively to a single surface magnetic layer (as in our experiments) or to multiple magnetic layers below the surface.

Let the bulk magnetization be given by $\sum_i M_i$, where $M_i$ is the magnetization of layer $i$ normalized to 1. We assume the time dependence of the layer magnetization to be $M_i(t) = 1 - \Delta M_i(F_i)e^{-t/\tau(F_i)}$. Due to the finite penetration depth of the pump light, each layer experiences a different effective fluence $F_i = F(1-R)e^{-z_i/\delta}$, where $F$ is the applied fluence, $z_i = i \times c/4$ with $c$ = 2.58 nm being the $c$-axis lattice constant, and $\delta$ = 100 nm [1] and $R$ = 0.2 [2] are respectively the penetration depth and reflectivity at the pump wavelength $\lambda$ = 1400 nm. We assume that $\Delta M_i(F_i)$ and $\tau(F_i)$ follow the curves shown in Fig. 1d and Fig. 3c of the main text respectively.

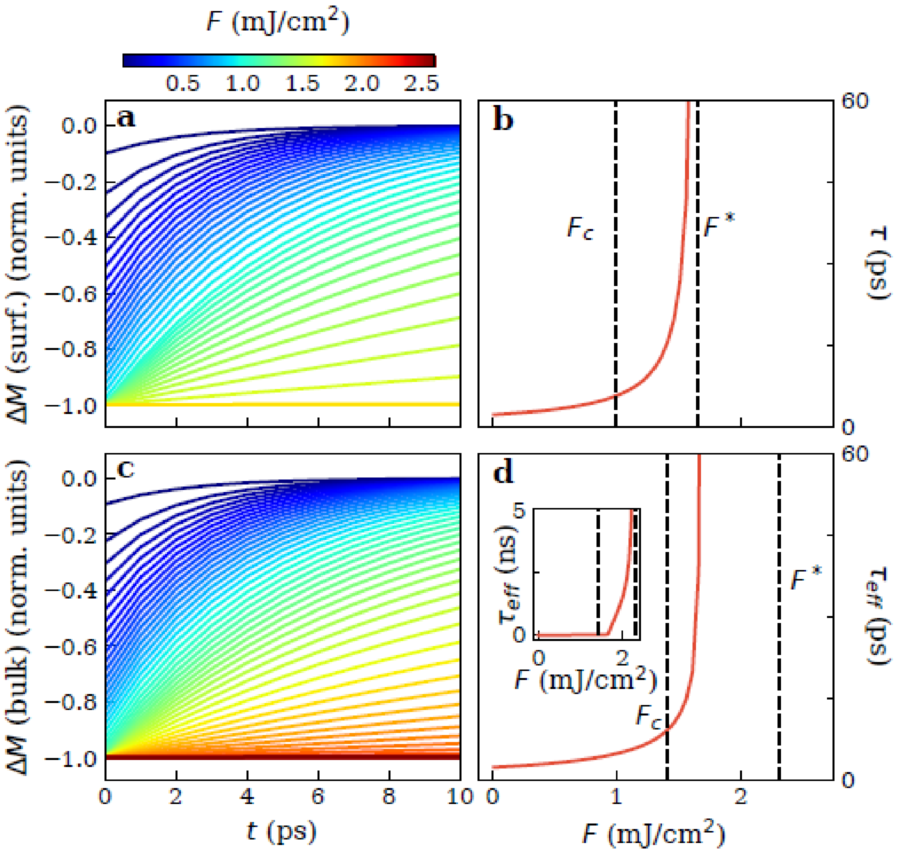


Figure S1: Simulated transient dynamics of **a,** the surface magnetization and **c**, the bulk magnetization for different applied pump fluences. **b** and **d** show the values of the relaxation constant $\tau$ extracted from fitting the curves in **a** and **b** respectively to a single exponential recovery. Vertical dashed lines indicate $F_c$ and $F^*$ for the surface and bulk. The inset in **d** shows the full range of $\tau_{eff}$ up to where it diverges at $F$*. The sudden upturn around $F$ = 1.6 mJ/cm$^2$ occurs where the fluence of the surface layer just reaches $F$*.

The transient magnetization dynamics are computed using the expression $\Delta M(t) = [M(t) - M(t^{<0})]/M(t^{<0})$, where $M(t) = \sum_i M_i(t)$ and $M(t^{<0})$ is the pre-

time zero magnetization. For the surface magnetization calculation, we only retain the $i$ = 0 term. Figures S1a and b show the fluence dependence of the simulated surface magnetization transients and the time constants extracted from fits to a single exponential, which follow the trends shown in Fig.3 of the main text by construction. For the bulk magnetization calculation, we restrict the sum to the first 48 layers (12 u.c.) to match the probe penetration depth at λ = 400 nm (δ = 31.25 nm). As shown in Fig. S1c and d, there are some key differences with the surface dynamics. First, based on our calculations, the critical fluences $F_c$ and $F^*$ are larger for the bulk case than for the surface case by a factor of $e^{z_i/\delta}$ with $i$ = 48 and δ = 100 nm. Second, the effective time constant $\tau_{eff}$ extracted from fits to a single exponential function exhibits a steep increase with fluence just above $F_c$, in contrast to the surface case where the steep increase occurs well above $F_c$. This arises because at the point where $F_c$ is reached throughout the bulk, the top layers already experience a fluence close to $F^*$ and contribute slow exponential terms to the sum over $i$. This makes the separation between $F_c$ and $F^*$ more difficult to resolve in the bulk case, and serves as a motivation for using a surface sensitive probe.

## S2. Time-resolved SHG transients in the presence of a magnetic field

Recent work [3] showed that when $Sr_2IrO_4$ is in the zero magnetic field – + + – state, the SHG signal is dominated by a surface electric-dipole (ED) contribution. On the other hand, in an in-plane magnetic field $H > H_c$ = 200 mT, there is a metamagnetic transition into a + + + + state [4], where the SHG signal becomes dominated by a bulk magnetization-induced magnetic-dipole (MD) contribution.

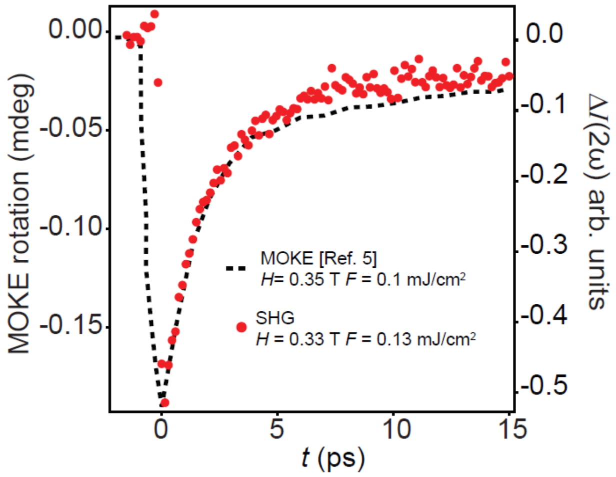


Figure S2. A comparison of in-field MOKE transients (adapted from Ref.[5]) and in-field SHG transients acquired under similar field and fluence.

We performed in-field ($H$ = 330 mT) time-resolved SHG-RA measurements on $Sr_2IrO_4$ using the short working-distance magnetic microstat apparatus described in Ref. [3]. As shown in Fig. S2, the in-field SHG transient acquired in the low fluence regime undergoes a prompt suppression and exponential recovery, reminiscent of our zero-field data. This verifies that photo-excitation is suppressing magnetic order in the bulk and not exclusively at the surface. We note that the dynamics reported in a recent ultrafast MOKE study [5] performed in the low fluence regime $F < 0.3$ mJ/cm$^2$ agree very well with our in-field SHG results (Fig. S2), which further confirms that both techniques are probing the recovery of + + + + order with bulk sensitivity.

## S3. Two- and three-temperature model results

Early pioneering work on laser-induced ultrafast demagnetization of ferromagnetic nickel introduced a three-temperature model (3TM) to explain its out-of-equilibrium dynamics [6]. This model assumes that immediately following photo-excitation, the electronic (*e*), lattice (*l*) and spin (*s*) subsystems form three thermalized reservoirs with independent temperatures and specific heats ($C_e$,$T_e$), ($C_l$,$T_l$) and ($C_s$,$T_s$), which interact via a set of coupling constants ($g_{el}$, $g_{es}$, $g_{sl}$) that control the rate of heat transfer between the different reservoirs. In such models, suppression of the magnetic ordering arises from a thermal effect related to an increase of $T_s$.

While such models are less applicable to insulating systems like $Sr_2IrO_4$, we nevertheless performed a 3TM analysis using the set of coupled differential equations below to explicitly show that such thermal effects cannot explain our observations in $Sr_2IrO_4$.

$$C_e(T_e)\frac{dT_e}{dt} = -g_{el}(T_e - T_l) - g_{es}(T_e - T_s)$$

$$C_l(T_l)\frac{dT_l}{dt} = g_{el}(T_e - T_l) - g_{ls}(T_l - T_s)$$

$$C_s(T_s)\frac{dT_s}{dt} = g_{es}(T_e - T_s) + g_{ls}(T_l - T_s)$$

The electronic heat capacity was taken to be $C_e = \gamma T_e$, with $\gamma = 2$ mJ/mol K$^2$ [7], the lattice heat capacity was modelled using a sixth order polynomial fit to the reported data in Ref. [7] and the spin specific heat was assumed to take the form predicted for a 2D spin-1/2 Heisenberg antiferromagnet [8]. Heat diffusion away from the probed region was not included in our model because it is much slower than the equilibration processes of interest. We assume that the pump pulse acts to instantaneously raise only $T_e$ by an amount:

$$T_e(t=0) = \sqrt{\frac{2 * F * (1-R)}{\delta * \gamma} + T_e(t<0)^2}$$

where *F* is the pump fluence, $R = 0.2$ [1] and $\delta = 100$ nm [2] are the sample reflectivity and penetration depth at $\lambda = 1400$ nm respectively. Both $T_l$ and $T_s$ are assumed to remain at the pre-pumped equilibrium temperature at $t = 0$.

We assumed a value of $5\times10^{12}$ W/mol-K for $g_{el}$, $g_{sl}$ and $g_{es}$, which is reasonable for real materials [9], in order to account for the following experimentally known features of $Sr_2IrO_4$: (i) There is substantial coupling between electronic, lattice and spin degrees of freedom within each Ir-O layer and so we treat them on equal footing; (ii) It produces a decay time of $T_e$ consistent with the observed timescale of $\tau_0$; (3) The system is fully equilibrated by $t = 10$ ps (at least for low fluences). We note that the relevant qualitative

trends exhibited by the 3TM (as described below) do not depend on the exact values chosen for $g_{el}$, $g_{sl}$ and $g_{es}$. Therefore, choosing a different set of values would not affect our conclusions. Solutions to the two-temperature model (2TM) involving only $T_e$ and $T_l$ can be obtained by simply setting $g_{es}$ and $g_{sl}$ to zero in our 3TM, which exhibit qualitatively similar behaviour.

Figure S3 shows the solution of the 3TM using several representative values of the pump fluence and $T = 80$ K. The following key features show why it cannot explain our experiments:

(i) $T_e$ far exceeds $T_N$ even for $F << F_c$, which indicates that the experimentally observed suppression of the MOP is not due to heating of the electronic subsystem.

(ii) $T_s$ begins to rise only after $T_e$ begins to fall. This is not compatible with our observations in Fig. 4a-c of the main text, which show that charge excitation and suppression of the MOP occur concurrently within our resolution.

(iii) There is no evidence for a slow relaxation timescale for $T_s$ or any anomaly in its relaxation rate within the 3TM, even at high fluences where $T_s$ crosses $T_N$. One can understand that this must be true simply by inspecting the equation governing the relaxation rate of $T_s$, namely $\frac{1}{C_s(T_s)}[g_{es}(T_e - T_s) + g_{ls}(T_l - T_s)]$. First, no divergence of $C_s$ has been observed at $T_N$ in specific heat measurements [7], which is naturally expected for $Sr_2IrO_4$ because $T_N$ is merely the temperature where already in-plane correlated 2D planes become locked along the $c$-axis. Much of the magnetic entropy is already lost far above $T_N$ where in-plane correlations develop. Second, the temperature differences $T_e - T_s$ and $T_l - T_s$ set a global scale for the system relaxation rate that cannot be erased by any internal dynamics of the magnons. Therefore, there is simply no mechanism for a diverging timescale in this model.

(iv) Higher pump fluence leads to a higher relaxation rate of $T_s$ for the reasons discussed above in (iii), which is opposite to the behavior observed for $\tau$. Note that this effect will be even more pronounced in the time dependence of $\Delta I(2\omega)$ because of the form of the nonlinear conversion function between $T_s$ and $\Delta I(2\omega)$ (Fig. 1c).

(v) For fluence values where $T_s$ begins to cross $T_N$ (Fig. S3b), one would expect the ED SHG signal to be zero during the time interval where $T_s > T_N$. Once $T_s$ dips back below $T_N$ the ED SHG signal should recover very fast because the SHG intensity is a steep function of temperature just below $T_N$. Such discontinuous features are not observed in our experiments.

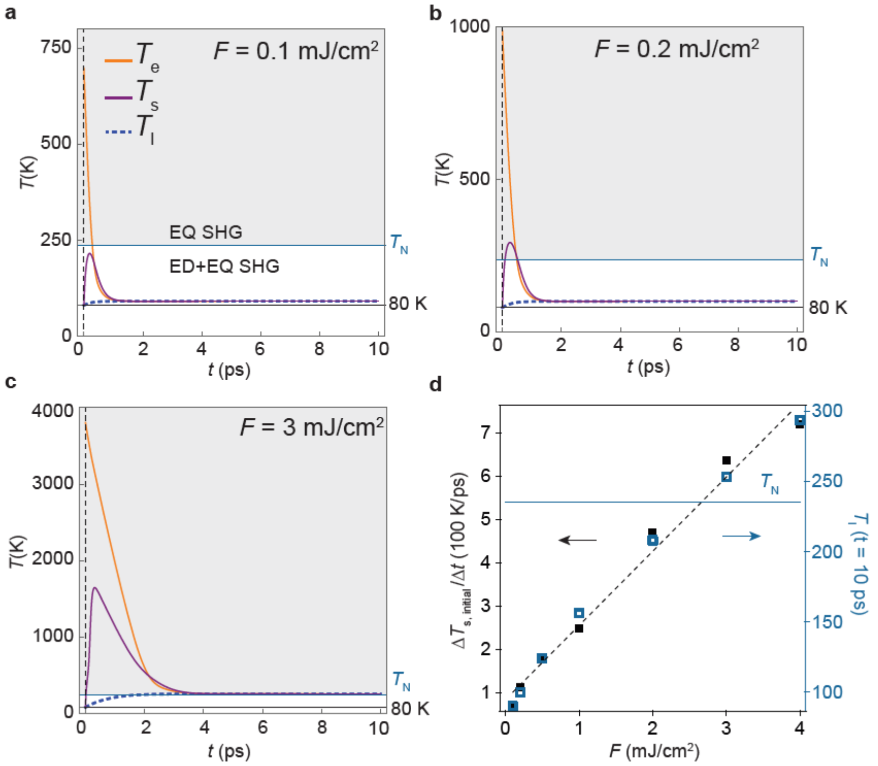


Figure S3. **a-c**, Solutions to the 3TM for an initial temperature $T$ = 80 K at representative $F$ values. White (gray) region denotes where one expects ED + EQ (just EQ) SHG contributions. The fluences corresponding to the three regimes in a-c will change depending on the chosen $g$ values, but the trends stay the same. **d,** The rate of change of $T_s$ extracted from a linear fit to the initial decay (< 1 ps) after the maximum (black), and the final equilibrated temperature (blue), plotted as a function of $F$.

## S4. Coherent in-plane magnon in the $F > F_c$ regime

We observe coherent oscillations of the in-plane magnon mode with symmetry $B_{2g}$ in the MOKE transients for $F > F_c$, albeit with a lifetime limited to several picoseconds, despite the absence of long-range inter-plane magnetic correlations. This in-plane magnon mode involves a precession of the $J_{eff} = 1/2$ moments out of the plane, which produces the observed oscillations in the MOKE transients [10] and does not depend on inter-plane magnetic correlations. This is consistent with previous time-resolved RIXS studies [11] and static RIXS measurements on La-doped $Sr_2IrO_4$ [12, 13] showing that in-plane magnon modes survive even in the absence of 3D long-range ordering, albeit with shorter lifetime. The source of these transient MOKE oscillations is not to be confused with the source of the static MOKE signal that occurs in finite magnetic field, which is sensitive to the bulk magnetization and thus *does* depend on having inter-plane + + + + magnetic correlations [5].

As discussed in Ref. [3], the zero-field SHG response is sensitive to the in-plane surface magnetization of the – + + – state. Since the in-plane magnon mode involves precession of the $J_{eff} = 1/2$ moments out of the plane, this will cause the in-plane projection of the magnetization to also oscillate, which should in principle be detectable by time-resolved SHG. However, unlike in MOKE, we do not observe coherent magnon induced oscillations in the transient SHG response likely for the following reasons. Since MOKE probes the out-of-plane moment ($\propto \sin\theta$) whereas SHG probes the in-plane moment ($\propto \cos\theta$), where $\theta$ is the small canting angle away from the plane, the MOKE and SHG signals scale like $\theta$ and $1 - \theta^2/2$ respectively. Moreover, our MOKE setup uses lock-in detection whereas the SHG does not. These differences make MOKE inherently more sensitive to the coherent $B_{2g}$ magnon oscillations compared to SHG.

## S5. Time-resolved SHG transients for *F* > *F**

As the quartic potential transforms into a parabolic potential above *F**, the internal dynamics of the magnetic degrees of freedom should again speed up above *F**. In principle, a probe capable of measuring magnetic excitation lifetimes in the paramagnetic regime (*F* > *F**) should detect such a speed up. However, our SHG-RA probe can only sense excitation lifetimes of the AFM order parameter, which is zero for *F* > *F**. Therefore, we expect the SHG transients to remain slow for all *F* greater than *F**, which is indeed what we observe (Fig. S4).

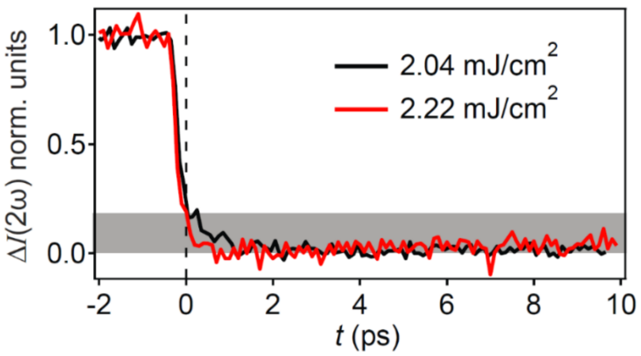


Figure S4. SHG transients acquired at $T$ = 80 K for fluences near and above $F^*$ ~ 1.6 mJ/cm$^2$ under the same conditions as shown in Fig. 3 a,b in the main text. The height of the grey bar denotes the excess EQ SHG intensity induced by magneto-elastic distortions.

We also elaborate on the possible explanation for the slower exponential drop after $t$ = 0 that is apparent at high fluences. In thermal equilibrium, $Sr_2IrO_4$ undergoes lattice deformations across $T_N$ due to magneto-elastic coupling [14, 4], which become more pronounced as the MOP increases. Therefore, below $T_N$, not only is there an onset of magnetization-induced ED SHG but also a change in the existing EQ SHG tensor elements induced by lattice deformations [15, 16]. Upon photo-excitation, one expects the lattice deformations to partially or fully relax in response to a partial or full melting of the MOP respectively. However, since the suppression of magnetic ordering by photo-doping occurs on a timescale (< 0.3 ps) that is much faster than the lattice relaxation time (~ 1-2 ps) [17, 18], the extent to which the lattice is able to relax will depend on the timescale τ for the MOP to recover. For example, if τ << 1-2 ps, then the lattice will not have sufficient time to relax and will thus be frozen in its initial state. Conversely, if τ >> 1-2 ps, then the lattice can relax to the full extent allowed by the transient value of the MOP. In our experiments, the regime where τ >> 1-2 ps is only achieved when *F* approaches *F**, which is why those SHG transients show the slow lattice relaxation component most clearly (Fig. S4). For lower fluences, not only does τ become shorter but the MOP also becomes suppressed by smaller amounts. Therefore, although a finite lattice relaxation component must still exist in this regime, it constitutes a much smaller fraction of the overall SHG signal, making it difficult to resolve.

## S6. Ruling out alternative explanations for slow dynamics

In this section we discuss other mechanisms that were considered towards explaining the slow recovery of the MOP in $Sr_2IrO_4$ and why they were ruled out.

*1. Near-degeneracy of different c-axis stacking arrangements* It has been reported that there are several stacking arrangements of the AFM ordered layers along the *c*-axis that may be close in energy and challenging to distinguish using diffraction based techniques alone [4, 19, 20, 21]. Therefore, one may ask whether after destroying *c*-axis magnetic correlations with the pump beam, the system, in the process of recovery, becomes trapped in some metastable stacking arrangement, which returns to the true ground state only through a slow annealing process. There are two arguments that can be used to rule out this scenario: (i) The *c*-axis correlations are destroyed at $F_c$, yet the recovery dynamics remain fast with no anomalous change at $F_c$; (ii) For the scenario proposed one would expect a discontinuous jump in the recovery time at the point where *c*-axis correlations are destroyed. However, we observe a power law type increase of $\tau$ upon approaching $F^*$, not a sudden jump.

*2. Healing of topological defects* Topological defects in an order parameter field created by spatially localized absorption of photons have recently been invoked to explain the slow recovery dynamics in photo-excited charge density wave materials [22]. However, time-resolved x-ray scattering measurements on $Sr_2IrO_4$ report no transient broadening of the magnetic diffraction peak and thus no reduced correlation length [11]. Moreover, if the suppression of the MOP in $Sr_2IrO_4$ was related to the presence of topological defects (vortex/anti-vortex pairs) in the spin texture created by the pump, then the defect density would be proportional to the pump fluence. However, the equilibration rate of topological defects (i.e., recombination rate of vortex/anti-vortex pairs), is proportional to their density. Therefore, one would expect that the recovery rate increases linearly with pump fluence. This is opposite to our observed behavior in $Sr_2IrO_4$, where the recovery rate decreases with pump fluence, which rules out this scenario.

Another scenario is related to the Kibble-Zurek mechanism [23] where topological defects are created as the system relaxes from the pump-induced paramagnetic state back into the AFM state. Here one would expect the recovery to suddenly become very slow once the system is pumped into the paramagnetic state. However, we do not observe any drastic slowing down of the recovery across $F_c$, ruling out this mechanism.

3. *Slow relaxation of the magneto-elastic deformation* We consider here a hypothetical scenario in which there is a critical lattice deformation amplitude above which magnetic long-range order is not supported. In this scenario, the critical amplitude would be reached when $F > F^*$, and the time required for the lattice to relax back below the critical amplitude thus becomes the bottleneck for the recovery of magnetic order. For the following reasons, we rule out this scenario. (1) If this scenario were correct, then one would expect a discontinuous jump in the SHG recovery time at $F^*$. Instead, we observe a power law increase upon approaching $F^*$. (2) If this scenario were correct, then one would expect the magnetization-induced ED SHG contribution to suddenly reappear at the instant the lattice relaxes across the critical amplitude, resulting in a discontinuity in the slope of the SHG transient. However, we do not observe any such discontinuity. (3) Recent studies show that magnetic order in $Sr_2IrO_4$ is robust against substantial lattice deformation imparted by both compressive and tensile epitaxial strain [24], applied uniaxial strain [25] and hydrostatic pressure up to ~17 GPa [26].

## S7. Details of the Langevin theory

We derive equations of motion for our magnetic degrees of freedom starting from a Hamiltonian by building on the standard approach to studying dynamical critical phenomena at finite temperature developed by Hohenberg and Halperin [27, 28]. To describe the thermalization of the $z$-axis magnons, we start with the following Hamiltonian:

$$H[\varphi] = \frac{1}{2}\int dz \left\{[\nabla_z \varphi(z,t)]^2 + \tau_0^{-1}\varphi^2(z,t) + \frac{\lambda}{2}\varphi^4(z,t)\right\}$$

where $\varphi(z,t)$ is a real bosonic scalar field that parameterizes how the intralayer Néel vector varies along the $z$-axis, $\tau_0^{-1}$ is a temperature-dependent mass term that is proportional to the deviation from the mean-field transition temperature, and $\lambda$ is a purely real coupling constant. The Hamiltonian can be expressed in terms of its Fourier components in the following way:

$$H[\varphi] = \frac{V}{2}\int \frac{dk}{2\pi}(k^2 + \tau_0^{-1})\varphi_{-k}\varphi_k + \frac{\lambda V}{4}\int \frac{dk_1}{2\pi}\int \frac{dk_2}{2\pi}\int \frac{dk_3}{2\pi}\varphi_{k_1}\varphi_{k_2}\varphi_{k_3}\varphi_{-k_1-k_2-k_3}$$

where $\varphi_k$ is the $k^{\text{th}}$ Fourier component of the order parameter field and $V$ is the volume. The relaxation dynamics of the system can then be studied through the Langevin equation:

$$\partial_t \varphi_k(t) = -\frac{1}{V}\frac{\delta\{H[\varphi_k(t)]\}}{\delta\varphi_{-k}(t)} + \xi_k(t)$$

where $\xi_k(t)$ is a Gaussian noise term with $\langle \xi_k(t)\rangle = 0$ and $\langle \xi_k(t)\xi_{k'}(t')\rangle = \delta(t-t')\delta(k+k')(k^2+\tau_0^{-1})[2n_k(t)+1]$, which describes fluctuations and imprints a non-equilibrium fluctuation-dissipation relation for some general distribution function $n_k(t)$. In the case of thermal equilibrium $n_k(t)$ is simply the Bose-Einstein distribution that, in the high temperature ($T$) limit, can be expanded as $2n_k(t) + 1 \approx 2T/(k^2+\tau_0^{-1})$, which is precisely the regime considered in the seminal work by Hohenberg and Halperin [27] (model A) where fluctuations are simply proportional to $T$. In our study, we keep the noise in this more general form that one would derive based on the Keldysh formalism. Explicitly writing out the Langevin equation leads to the form shown in the manuscript:

$$\partial_t \varphi_k(t) = -(k^2+\tau_0^{-1})\varphi_k(t) - \lambda\int \frac{dk_1}{2\pi}\int \frac{dk_2}{2\pi}\ \varphi_{k_1}(t)\varphi_{k_2}(t)\varphi_{k-k_1-k_2}(t) + \xi_k(t)$$

Starting from this equation, the first-order perturbative (Hartree shift) correction to the mass (i.e. the relaxation time) is given by $\tau^{-1} = \tau_0^{-1} - \lambda\int d\omega\rho(\omega)n(\omega) = \tau_0^{-1} - \lambda N_{mag}$, where $\rho(\omega)$ is the magnon density of states, $n(\omega)$ is their distribution function versus energy $\omega$, and $N_{mag}$ is the total number of magnons. In thermal equilibrium, increasing temperature increases the magnon number and thus also the decay time, with the thermal critical point located at $\tau^{-1} = 0$.

We are specifically interested in studying a general magnon distribution function $n_k(t)$ that is non-thermal and changes in time following the linearized Boltzmann equation:

$$\partial_t n_k(t) = -|\tau^{-1}|[n_k(t) - n_k^T]$$

where $n_k^T$ is the equilibrium Bose-Einstein distribution function at temperature $T$ and $\tau$ is the thermalization time. We note that the distribution function of course describes a fully 3D system and so ordering is allowed at finite temperatures. But since the rate-limiting step is thermalization along the $z$-axis, we are defining $n_k(t)$ as the distribution function after integrating out the $x$ and $y$ components. This equation governs how quickly an out-of-equilibrium magnon distribution function thermalizes back to Bose-Einstein form for some fixed energy content corresponding to temperature *T*. Up to leading order, the lifetime of a magnetic excitation (given by the mass of the potential expressed in the Hamiltonian above) is also the average lifetime of a deviation from the Bose-Einstein distribution function. This can be rigorously proven through a systematic derivation of the Boltzmann equation using the Keldysh formalism, which shows that the relaxation time in a linearized Boltzmann equation in general is given by the imaginary part of the retarded self-energy [for details see for example Ref. [29] sec. V.B.; Ref [30] sec. 3.5; Ref [31] sec. III]. This means that the timescale $\tau$ found in the Boltzmann equation is equivalent to the $\tau$ derived from our Hamiltonian. For $\tau > 0$ the magnons want to enter the ordered phase with an order parameter $\langle\varphi\rangle \sim 1/\sqrt{\tau\lambda}$. Note that one would typically expect the order parameter to be defined by $1/\sqrt{\tau\lambda}$ in equilibrium (i.e. when $\tau$ is time independent).

An interesting consequence of these equations is that the relaxation time (and therefore the distance to the critical point) is susceptible to the number of magnons in the system but not to the total energy in the system. In thermal equilibrium, there is, of course, a one-to-one correspondence between the total magnon number ($N_{mag}$) and total magnon energy ($E_{mag}$), related through the temperature of the system *T*. For a generic density of states of the form:

$$\rho(\omega) = \rho_0 \omega^\alpha$$

for some power $\alpha > 1$ (again the system is physically three-dimensional), the magnon number and energy are given by:

$$N_{mag} = \rho_0 T^{1+\alpha} f(\alpha)$$
$$E_{mag} = \rho_0 T^{2+\alpha} f(\alpha + 1)$$

where $f(\alpha) = \alpha\Gamma(\alpha)\zeta(\alpha+1)$, with $\zeta(\alpha)$ the Riemann zeta-function and $\Gamma(\alpha)$ the gamma-function. In thermal equilibrium, $N_{mag}$ and $E_{mag}$ are related such that they yield the same value for *T*. In stark contrast, when driven away from equilibrium, $N_{mag}$ and $E_{mag}$ are not constrained to be related via the Bose-Einstein distribution anymore and the two equations may define two different effective temperatures, which we call $T_{num}$ and $T_{en}$ respectively. To illustrate the consequences of this behaviour in an intuitive way and show how it explains our experimental observations, we consider the three different regimes of our experiment and a simplified out-of-equilibrium distribution for the magnon degrees of freedom:

(1) **Initial $t < 0$ regime** before the system is pumped: the magnons are in thermal equilibrium at an initial temperature $T_i$ below the 3D AFM ordering temperature $T_N$ and are described by a Bose-Einstein distribution $n^{B.E.}(\omega/T_i)$.

(2) **Quenched regime** immediately after the pump pulse is switched off: the pump creates a large density of magnons through the charge relaxation process, which modifies its distribution function. For ease of calculation, we assume that immediately after the pumping stage, the magnon distribution is $n(\omega) = n^{B.E.}(\omega/T_i) + N_{pump}\,\delta(\omega - \omega_0)$ , i.e. it has an extra number of magnons $N_{pump}$ at some energy $\omega_0$ introduced by the pump beam. But our results are valid for general more complicated non-equilibrium distribution functions. This leads to the following expressions:

$$N_{mag} = \rho_0 T_i^{1+\alpha} f(\alpha) + N_{pump}\rho_0\omega_0^{\alpha} \equiv \rho_0 T_{num}^{1+\alpha} f(\alpha)$$

$$E_{mag} = \rho_0 T_i^{2+\alpha} f(\alpha+1) + N_{pump}\rho_0\omega_0^{\alpha+1} \equiv \rho_0 T_{en}^{2+\alpha} f(\alpha+1)$$

where we defined the corresponding effective temperatures associated with the magnon number and energy. In principle $T_{num} \neq T_{en}$. Since $T_{num} > T_i$, the order parameter is suppressed.

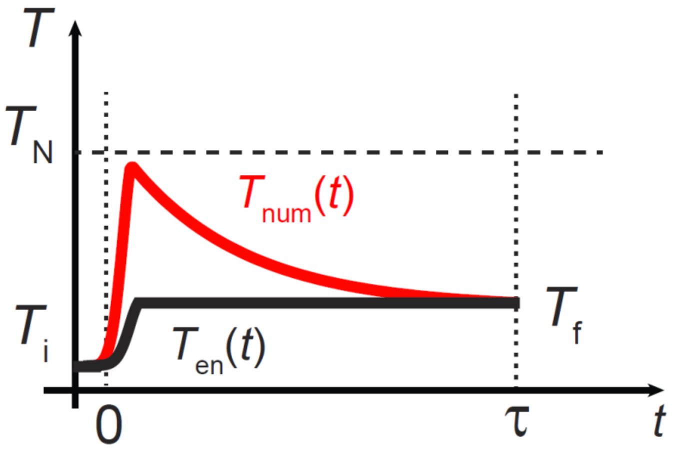


Figure S5. Schematic of the temporal evolution of the effective temperatures $T_{num}$ and $T_{en}$ after pump excitation corresponding to the experimental regime $F < F^*$. The peak in the temperature curves occur after magnons are emitted following charge relaxation, hence they are delayed from $t = 0$.

(3) **Relaxation regime**: Magnon collisions lead to equilibration between the different magnon modes, which allows the magnon distribution function to relax back towards a Bose-Einstein distribution $n^{B.E.}(\omega/T_f)$, albeit at a higher final temperature $T_f$. Since the energy is conserved this must be $T_f = T_{en}$. After relaxation, $N_{mag}$ and $E_{mag}$ are again determined by the same temperature $T_f$. The three stages can be expressed via the effective temperature in the magnon particle number $T_i \rightarrow T_{num} \rightarrow T_{en}$ (Fig. S5). The key insight in the proposed mechanism is that $T_{num}$ can be brought rather close to the critical temperature $T_N$ through pumping while both $T_i$ and $T_{en}$ remain below $T_N$. Thus, the system becomes trapped in a non-equilibrium critical state that suppresses the relaxation of the out-of-equilibrium magnon distribution, although the energy density is far from criticality. This is precisely the situation realized in our experiments near $F^*$. Both equilibria (before and long after the pump) are non-critical (see section S3), yet the intermediate non-equilibrium state mimics criticality for a transient time regime. The equilibration times can be explicitly solved in this simplified model to yield:

$$\tau^{-1}(t<0)=\tau_0^{-1}-\lambda\int d\omega\rho(\omega)n^{B.E.}(\omega/T_i)$$

$$\tau^{-1}(t>0)=\tau^{-1}(t<0)-\lambda N_{pump}\rho(\omega_0)$$

$$\tau^{-1}(t\gg 0)=\tau_0^{-1}-\lambda\int d\omega\rho(\omega)n^{B.E.}(\omega/T_f)$$

The effect observed in our experiments can be seen through the expression for $\tau^{-1}(t>0)$, which shows that at some critical pump intensity (corresponding to $F^*$ in our experiments), the relaxation rate goes to zero. The physical picture behind this mechanism is the following: Photo-doping occurs immediately upon pump excitation and causes a reduction of the magnetic order parameter in proportion to the number of photo-carriers. In contrast, the magnon number is proportional to the energy released when the photo-carriers subsequently decay. This means that the critical fluences for collapsing the magnetic order via photo-doping and magnon generation, $F_c$ and $F^*$ respectively, are generally different. The relaxation of the photo-carriers populates magnon modes around $\omega\approx\omega_0$. Now the system wants to relax towards its equilibrium state. This happens via local scattering processes that both generate magnon modes ("in-scattering") and destroy magnon modes ("out-scattering"). For a system away from a critical point, out-scattering into the continuum is typically much larger and the system acquires an effective mass. Here, however, the huge population of magnon modes around $\omega\approx\omega_0$ leads to a compensation of in- and out-scattering, i.e., to a temporarily vanishing mass. Only when the magnon peak has considerably decayed is the mass effectively restored. Since the relaxation rate of the 3D AFM order parameter is given exactly by the mass, it is restored on the same slow timescale.

To verify that a regime where $T_{num} > T_{en}$ as shown in Fig. S5 indeed exists, we write out the formal expression for $N_{mag}$ and $E_{mag}$ in our model above to find:

$$T_{num}=T_i\left(1+\frac{N_{pump}\omega_0^{\alpha}}{T_i^{\alpha+1}f(\alpha)}\right)^{\frac{1}{\alpha+1}}$$

$$T_{en}=T_i\left(1+\frac{N_{pump}\omega_0^{\alpha+1}}{T_i^{\alpha+2}f(\alpha+1)}\right)^{\frac{1}{\alpha+2}}$$

Defining $X=\frac{N_{pump}\omega_0^{\alpha}}{T_i^{\alpha+1}f(\alpha)}$ and $y=\frac{\omega_0}{T_i}$, the condition for $T_{num} > T_{en}$ becomes

$$\left(1+Xy\frac{f(\alpha)}{f(\alpha+2)}\right)^{\frac{\alpha+1}{\alpha+2}}<1+X$$

Since $\frac{\alpha+1}{\alpha+2}<1$, there is always an $X_c$ such that for $X>X_c$, the above condition is satisfied.

## S8. Restoration of the initial SHG-RA pattern after relaxation

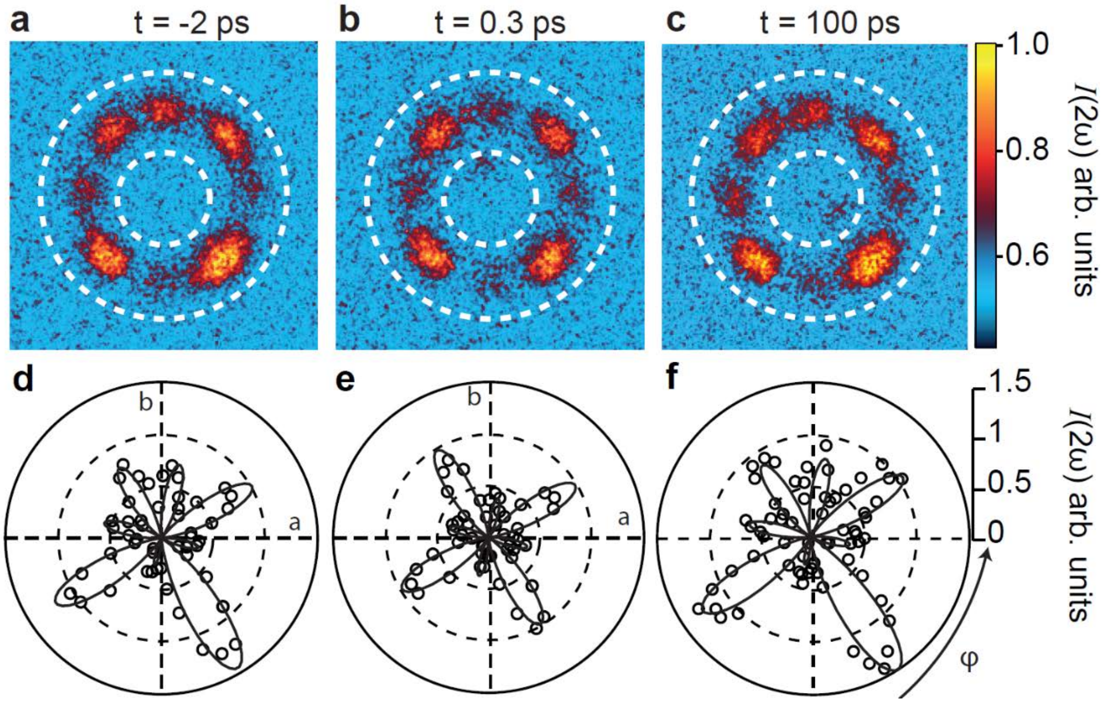


Figure S6. Raw SHG-RA data acquired from a single magnetic domain ($T$ = 80 K) in $P_{in}$-$S_{out}$ geometry with $n_{ex}$ = 0.095 at **a,** $t$ = - 2 ps, **b,** $t$ = 0.3 ps and **c,** $t$ = 100 ps. Radially integrated data are shown below in **d**, **e**, and **f**. Recovery of the initial magnetic order (compare **d** and **f**) is observed. Solid lines are fits to the ED and EQ SHG expressions described in the main text.

In zero magnetic field, there are four energetically equivalent magnetic domains in $Sr_2IrO_4$, corresponding to four possible orientations of the surface ferromagnetic moment and thus four possible orientations of the large SHG lobe [32, 3]. To ensure that the original magnetic order and domain orientation is recovered even after pumping to above $F^*$, we focus our pump and probe beams inside a single domain, identified via SHG imaging. To verify this, we show instantaneous SHG-RA data acquired for $F > F^*$ before, immediately after and long after pump excitation in Fig. S6. To convert the raw CCD images into polar SHG-RA plots, data were radially integrated between the white dashed lines. Clearly the original domain orientation is recovered by $t$ = 100 ps.

We note that the same magnetization-induced surface ED response can in principle arise from alternative stacking orders such as + + + + and – + – +. However, the former generates an additional strong bulk magnetic-dipole SHG term because it possesses a net bulk magnetization [3], and the latter allows an additional bulk electric-dipole SHG term because it breaks inversion symmetry. Since we do not observe a transient appearance of additional SHG contributions upon pumping, we can also rule out a change from – + + – to one of these alternative stacking orders.

## S9. Time-resolved SHG transients for different polarization channels

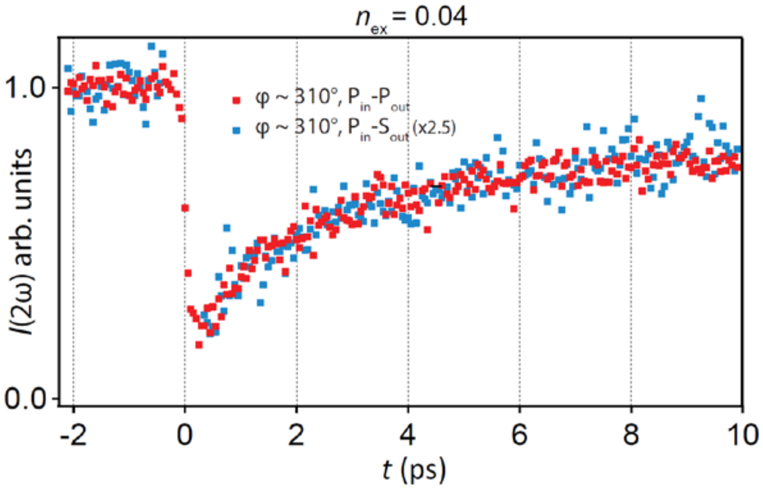


Figure S7. SHG intensity versus time acquired at a fixed value of pump fluence and scattering plane angle φ for two different polarization geometries, which show identical relaxation dynamics.

The SHG dynamics observed in Fig. 3 of the main text were consistently observed under different polarization geometries and different scattering plane angles. Figure S7 shows a direct comparison of the SHG transient acquired under $P_{in}$-$S_{out}$ and $P_{in}$-$P_{out}$ geometries. This is expected since all elements of the ED SHG tensor are proportional to the MOP.

## Bibliography


[1] Lee, J. S., Krockenberger, Y., Takahashi, K. S., Kawasaki, M. & Tokura, Y. Insulator-metal transition driven by change of doping and spin-orbit interaction in $Sr_2IrO_4$. *Phys. Rev. B.* **85**, 035101 (2012).

[2] Nichols, J. *et al.* Anisotropic electronic properties of *a* -axis-oriented $Sr_2IrO_4$ epitaxial thin-films. *Appl. Phys. Lett.* **103**, 131910 (2013)

[3] Seyler, K.L *et al*, "Spin-orbit-enhanced magnetic surface second-harmonic generation in $Sr_2IrO_4$," Phys. Rev. B102, 201113 (R) (2020).

[4] Porras, J. *et al.* Pseudospin-lattice coupling in the spin-orbit Mott insulator $Sr_2IrO_4$. *Phys. Rev. B* **99**, 085125 (2019).

[5] Afanasiev, D. *et al.* Ultrafast Spin Dynamics in Photodoped Spin-Orbit Mott Insulator $Sr_2IrO_4$. *Phys. Rev. X* **9**, 021020, (2019).

[6] Beaurepaire, E., Merle, J.-C., Daunois, A. & Bigot, J.-Y. Ultrafast Spin Dynamics in Ferromagnetic Nickel. *Phys. Rev. Lett.* **76**, 4250 (1996).

[7] Kini, N. S., Strydom, A. M., Jeevan, H. S., Geibel, C. & Ramakrishnan, S. Transport and thermal properties of weakly ferromagnetic $Sr_2IrO_4$. *J. Phys. Condens. Matter* **18**, 8205–8216 (2006).

[8] Hofmann, M. *et al.* Evidence for a large magnetic heat current in insulating layered cuprates. *Phys. Rev. B* **67**, 184502 (2003).

[9] Shen, X., Timalsina, Y. P., Lu, T.-M. & Yamaguchi, M. Experimental study of electron-phonon coupling and electron internal thermalization in epitaxially grown ultrathin copper films. *Phys. Rev. B* **91**, 045129 (2015).

[10] Seifert, U. F. P. & Balents, L. Optical excitation of magnons in an easy-plane antiferromagnet: Application to $Sr_2IrO_4$. *Phys. Rev. B* **100**, 125161 (2019).

[11] Dean, M. P. M. *et al.* Ultrafast energy- and momentum-resolved dynamics of magnetic correlations in the photo-doped Mott insulator $Sr_2IrO_4$. *Nat. Mater.* **15**, 601–605 (2016); Krupin, O. *et al.*, Ultrafast dynamics of localized magnetic moments in the unconventional Mott insulator $Sr_2IrO_4$, *J. Phys.: Condens. Matter* 28 32LT01 (2016).

[12] Gretarsson, H. *et al.* Persistent Paramagnons Deep in the Metallic Phase of $Sr_{2-x}La_xIrO_4$. *Phys. Rev. Lett.* **117**, 107001 (2016).

[13] Pincini, D. *et al.* Anisotropic exchange and spin-wave damping in pure and electron-doped $Sr_2IrO_4$. *Phys. Rev. B* **96**, 075162 (2017).

[14] Bhatti, I. N., Rawat, R., Banerjee, A. & Pramanik, A. K. Temperature evolution of magnetic and transport behavior in 5d Mott insulator $Sr_2IrO_4$: Significance of magneto-structural coupling. *J. Phys. Condens. Matter* **27**, (2014).

[15] Ron, A., Zoghlin, E., Balents, L., Wilson, S. D. & Hsieh, D. Dimensional crossover in a layered ferromagnet detected by spin correlation driven distortions. *Nat. Commun.* **10**, 1654, (2019).

[16] Bauer, K.-D. & Hingerl, K. Bulk quadrupole contribution to second harmonic generation from classical oscillator model in silicon. *Opt. Express* **25**, 26567 (2017).

[17] Li, R. *et al.* Ultrafast time-resolved structural changes of thin-film ferromagnetic metal heated with femtosecond optical pulses. *J. Chem. Phys.* **151**, (2019).

[18] Li, R. *et al.* Transient lattice deformations of crystals studied by means of ultrafast time-resolved x-ray and electron diffraction. *Struct. Dyn.* **5**, (2018).

[19] Clancy, J. P. *et al.* Dilute magnetism and spin-orbital percolation effects in $Sr_2Ir_{1-x}Rh_xO_4$. *Phys. Rev. B* **89**, 054409 (2014)

[20] Di Matteo, S. & Norman, M. R. Magnetic ground state of $Sr_2IrO_4$ and implications for second-harmonic generation. *Phys. Rev. B* **94**, 075148 (2016)

[21] Kim, B. J. *et al.* Phase-Sensitive Observation of a Spin-Orbital Mott State in $Sr_2IrO_4$. *Science.* **323**, 1329–1332 (2009)

[22] Zong, A. *et al.* Evidence for topological defects in a photoinduced phase transition. *Nat. Phys.* **15**, 27 (2019).

[23] Zurek, W. H. Cosmological experiments in condensed matter systems. *Phys. Rep.* **276**, 177–221 (1996).

[24] Kim, J. W. *et al.* Controlling symmetry of spin-orbit entangled pseudospin state through uniaxial strain. *Phys. Rev. B* **102**, 054420 (2020).

[25] Paris, E. *et al.* Strain engineering of the charge and spin-orbital interactions in $Sr_2IrO_4$. *PNAS* **117**, 24764 (2020).

[26] Haskel, D. *et al.* Possible Quantum Paramagnetism in Compressed $Sr_2IrO_4$. *Phys. Rev. Lett.* **124**, 67201 (2020).

[27] Hohenberg, P. C. & Halperin, B. I. Theory of dynamic critical phenomena. *Rev. Mod. Phys.* **49**, 435–479 (1977).

[28] Dolgirev, P. E., Michael, M. H., Zong, A., Gedik, N. & Demler, E. Self-similar dynamics of order parameter fluctuations in pump-probe experiments. *Phys. Rev. B* **101**, 174306 (2020).

[29] Sieberer, L. M., Buchhold, M. & Diehl, S. Keldysh field theory for driven open quantum systems. *Reports Prog. Phys.* **79**, 096001 (2016).

[30] Kamenev, A. & Levchenko, A. Keldysh technique and non-linear σ-model: basic principles and applications. *Adv. Phys.* **58**, 197–319 (2009).

[31] Kamenev, A. Many-body theory of non-equilibrium systems. *arXiv:cond-mat/0412296* (2004).

[32] Zhao, L. *et al.* Evidence of an odd-parity hidden order in a spin-orbit coupled correlated iridate. *Nat. Phys.* **12**, 32–36 (2016).
